# Supplementary material for: Automating DBSCAN via Deep Reinforcement Learning
Source: arXiv:2208.04537 source file (2022-08-09)
Supplement: Supplementary file 1 [file Appendix.tex]

%\clearpage
%\section{METHODS}\label{sec:appendix1}

\begin{figure}[t]
\centering
\includegraphics[width=9.0cm]{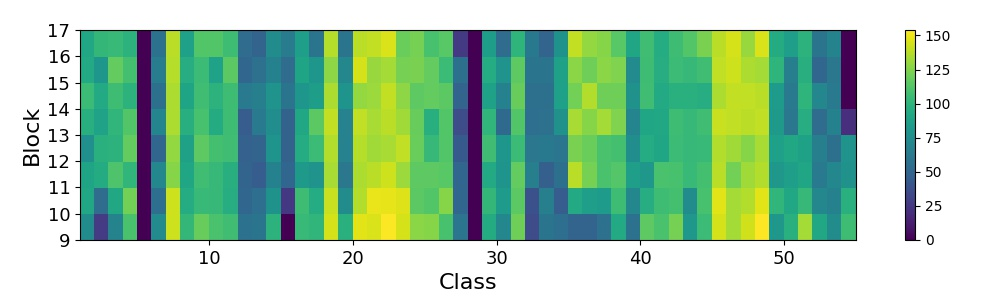}\vspace{-1em}
\centering
\caption{Cluster distribution on online dataset.}\label{fig:dataset}
\vspace{-1.2mm}
\end{figure}

\begin{table}[t]
    \caption{Glossary of Notations.}\label{table:notations}\vspace{-1em}
    \resizebox{\linewidth}{!}{%
    \begin{tabular}{r|p{6.7cm}}  
    \toprule
      %\hline\hline
      \textbf{Notation} & \textbf{Description}\\
      \hline
      $v_{j}$; $\mathcal{V}$ & The $j$-th object in data block; Data block\\
      $x_{j}$; $\mathcal{X}$; $d$& Feature of the $j$-th object of data block; Feature set; Feature dimension\\
      $y_{j}$; $\mathcal{Y}'$ & Label of the $j$-th object of data block; Partial label set\\
      $c_{n}$; $\mathcal{C}$ & The $n$-th cluster; Cluster set\\
      \hline
      $i$; $I$; $I_{max}$ & Step; End step; Maximum step\\
      $e$; $E$; $E_{max}$ & Episode; End episode; Maximum episode\\
      $l$; $L$; $L_{max}$ & Layer; End layer; Maximum layer\\
      $a^{(i)(e)}$; $\mathcal{A}$  & Action of the $i$-th step at episode $e$; Action space\\
      $s^{(i)(e)}$; $\mathcal{S}$ & State of the $i$-th step at episode $e$; State set\\
      $r^{(i)(e)}$; $R$ & Reward of the $i$-th step at episode $e$; Reward function\\
      $\mathcal{P}$; $\mathcal{P}_{o}$ & Parameter combination; Optimal parameter combination\\
      $B_{p}$ & Parameter space boundary of the parameter $p$\\
    \bottomrule
    \end{tabular}}
    \vspace{-2.5mm}
\end{table}

\begin{table*}[t]
    \setlength{\abovecaptionskip}{0.cm}
    \setlength{\belowcaptionskip}{-0.cm}
    \caption{Online evaluation and comparison in Predictive Mode.}\label{tab:complexity}
    \centering
    \scalebox{1.0}{
        \begin{tabular}{c|c|cc|cccc|cc|ccc}
        \hline
        \multirow{2}*{\textbf{Blocks}} & \multirow{2}*{\textbf{Metrics}} & \multicolumn{2}{c|}{\textbf{Traditional}} & \multicolumn{4}{c|}{\textbf{Evolutionary}} & \multicolumn{4}{c}{\textbf{Dedicated}} \\
        \cline{3-13}
         & & \multirow{1}*{\textbf{Rand}} & \multirow{1}*{\textbf{BO-TPE}} & \multirow{1}*{\textbf{Anneal}} & \multirow{1}*{\textbf{PSO}} & \multirow{1}*{\textbf{GA}} & \multirow{1}*{\textbf{DE}} & \multirow{1}*{\textbf{KDist}} & \multirow{1}*{\textbf{BDE}} & \multirow{1}*{\textbf{DRL_{all}}} & \multirow{1}*{\textbf{DRL_{one}}} & \\
        \hline
        \hline 
        \rowcolor{gray!15} $\mathcal{V}_{9}$  & NMI & .34±.31 & .49±.33 & .22±.34 & .14±.29 & .27±.37 & .10±.26 & .00±.00 & .00±.00 & \textbf{.68±.30} & \textbf{.68±.30}  & $\uparrow$ .19\\
        \rowcolor{white!15}                   & ARI & .10±.16 & .18±.20 & .07±.12 & .03±.11 & .11±.18 & .05±.15 & .00±.00 & .00±.00 & \textbf{.36±.20} & \textbf{.36±.20}  & $\uparrow$ .18\\
        \rowcolor{gray!15} $\mathcal{V}_{10}$ & NMI & .11±.14 & .28±.17 & .17±.21 & .24±.01 & .20±.21 & .12±.18 & .00±.00 & .00±.00 & \textbf{.33±.16} & \textbf{.33±.15}  & $\uparrow$ .05\\
        \rowcolor{white!15}                   & ARI & .00±.01 & .02±.02 & .01±.02 & .01±.02 & .01±.01 & .01±.02 & .00±.00 & .00±.00 & \textbf{.03±.02} & \textbf{.03±.02}  & $\uparrow$ .01\\
        \rowcolor{gray!15} $\mathcal{V}_{11}$ & NMI & .16±.15 & .29±.24 & .23±.18 & \textbf{.33±.29} & .23±.23 & .02±.05 & .00±.00 & .00±.00 & .30±.13 & \underline{.32±.08}  & - \\
        \rowcolor{white!15}                   & ARI & .01±.01 & \textbf{.02±.02} & .01±.01 & .00±.01 & .01±.02 & .00±.00 & .00±.00 & .00±.00 & .01±.01 & \textbf{.02±.00}  & - \\
        \rowcolor{gray!15} $\mathcal{V}_{12}$ & NMI & .23±.25 & .19±.24 & .10±.22 & \underline{.38±.26} & .34±.27 & .03±.06 & .00±.00 & .00±.00 & \underline{.38±.17} & \textbf{.46±.09}  & $\uparrow$ .08\\
        \rowcolor{white!15}                   & ARI & .01±.02 & .02±.04 & .01±.02 & .01±.03 & \textbf{.04±.06} & .00±.00 & .00±.00 & .00±.00 & .02±.01 & \underline{.03±.01}  & - \\
        \rowcolor{gray!15} $\mathcal{V}_{13}$ & NMI & .58±.35 & \underline{.70±.24} & .47±.40 & .44±.31 & .36±.28 & .08±.14 & .00±.00 & .00±.00 & .68±.34 & \textbf{.70±.27}  & - \\
        \rowcolor{white!15}                   & ARI & .31±.35 & .33±.28 & .21±.25 & .07±.16 & .08±.16 & .00±.00 & .00±.00 & .00±.00 & \textbf{.39±.29} & \underline{.37±.25}  & $\uparrow$ .06\\
        \rowcolor{gray!15} $\mathcal{V}_{14}$ & NMI & .36±.19 & .34±.28 & .47±.35 & .37±.33 & .27±.25 & .11±.24 & .00±.00 & .00±.00 & \underline{.60±.27} & \textbf{.62±.16}  & $\uparrow$ .15\\
        \rowcolor{white!15}                   & ARI & .03±.04 & .07±.15 & \textbf{.14±.17} & .06±.09 & .06±.12 & .03±.11 & .00±.00 & .00±.00 & \textbf{.14±.08} & .11±.07  & - \\
        \rowcolor{gray!15} $\mathcal{V}_{15}$ & NMI & .45±.35 & .38±.36 & .37±.33 & .30±.34 & .36±.32 & .09±.18 & .00±.00 & .00±.00 & \underline{.64±.28} & \textbf{.70±.03}  & $\uparrow$ .25\\
        \rowcolor{white!15}                   & ARI & .13±.14 & .17±.26 & .14±.24 & .06±.13 & .10±.17 & .00±.01 & .00±.00 & .00±.00 & \textbf{.21±.19} & \underline{.15±.05}  & $\uparrow$ .04\\
        \rowcolor{gray!15} $\mathcal{V}_{16}$ & NMI & .22±.32 & .45±.24 & .32±.29 & .19±.27 & .36±.27 & .12±.20 & .00±.00 & .00±.00 & \textbf{.60±.27} & \underline{.53±.20}  & $\uparrow$ .15\\
        \rowcolor{white!15}                   & ARI & .07±.15 & \underline{.10±.19} & .06±.12 & .00±.01 & .05±.09 & .00±.01 & .00±.00 & .00±.00 & \textbf{.17±.13} & .07±.06  & $\uparrow$ .07\\

        \hline
        \hline
        \end{tabular}
    }
\end{table*}

\begin{table}[h]
    \setlength{\abovecaptionskip}{0.cm}
    \setlength{\belowcaptionskip}{-0.cm}
    \caption{Time Complexity Analysis.}\label{tab:complexity}
    \centering
    \scalebox{1.0}{
        \begin{tabular}{c|cc}
        \hline
        Method & Type & Complexity\\
        \hline
        GA & Genetic Algorithm &\\
        PSO & Particle Swarm Optimization &\\
        ACO & Ant Colony Optimization &\\
        \hline
        SMAC & Bayesian Optimization & $O(nlogn)$\\
        Randomly & Randomly Optimization &\\
        \hline
        V-DBSCAN & K Disatance &\\
        BDE-DBSCAN & Binary Differential Evolution & $O(nlogn)$\\
        \hline
        {\framework} & Reinforcement Learning & $O(log)$\\
        \hline
        \end{tabular}
    }
\end{table}

\begin{table*}[t]
    \setlength{\abovecaptionskip}{0.cm}
    \setlength{\belowcaptionskip}{-0.cm}
    \caption{The comparison results of different parameter search method.}\label{tab:complexity}
    \centering
    \scalebox{1.0}{
        \begin{tabular}{c|c|cc|cccc|cc|c}
        \hline
        \multirow{2}*{\textbf{Dataset}} & \multirow{2}*{\textbf{Metrics}} & \multicolumn{2}{c|}{\textbf{Traditional}} & \multicolumn{4}{c|}{\textbf{Evolutionary}} & \multicolumn{3}{c}{\textbf{Dedicated}} \\
        \cline{3-11}
         &  & \multirow{1}*{\textbf{Rand}} & \multirow{1}*{\textbf{BO-TPE}} & \multirow{1}*{\textbf{Anneal}} & \multirow{1}*{\textbf{PSO}} & \multirow{1}*{\textbf{GA}} & \multirow{1}*{\textbf{DE}} & \multirow{1}*{\textbf{KDist}} & \multirow{1}*{\textbf{BDE}} & \multirow{1}*{\textbf{DRL}} \\
        \hline
        \hline 
        \multirow{7}*{Pathbased} & \rowcolor{gray!15} NMI (\%) & 59±24 & 75±14 & 35±33 & 47±28 & 44±32 & 11±21 & 0 & 0 & \textbf{75±21} \\
        & \rowcolor{gray!15} AMI (\%) & 59±24 & 75±14 & 35±33 & 41±33 & 43±32 & 11±20 & 0 & 0 & \textbf{75±21} \\
        & \rowcolor{gray!15} ARI (\%) & 57±31 & 78±16 & 29±36 & 37±36 & 38±38 & 7±18 & 0 & 0 & \textbf{77±26} \\
        %\cline{2-11}
        & $Eps$ & .15±.08  & .14±.04 & .41±.23 & .26±.30 & .28±.28 & .45±.29 & 0 & 0 & \textbf{.11±.03} \\
        & $MinPts$ & 47±44 & 50±28 & 151±83 & 88±94 & 98±74 & 164±78 & 0 & 0 & \textbf{28±10} \\
        & No. Cluster & 3±0 & 3±0 & 2±1 & 51±106 & 2±1 & 2±1 & 0 & 0 & \textbf{3±0} \\
        & First Iteration & 19±14 & 25±12 & 27±17 & 24±17 & 20±14 & 10±20 & 0 & 0 & \textbf{19±7} \\
        & All Iteration & 50±0 & 50±0 & 50±0 & 52±0 & 53±0 & 57±0 & 0 & 0 & \textbf{48±8} \\
        \hline
        \hline
        \multirow{7}*{Compound} & \rowcolor{gray!15} NMI (\%) & 63±27 & 72±7 & 58±31 & 53±37 & 56±27 & 21±33 & 0 & 0 & \textbf{79±4} \\
        & \rowcolor{gray!15} AMI (\%) & 62±27 & 72±7 & 57±31 & 52±36 & 54±28 & 20±33 & 0 & 0 & \textbf{79±4} \\
        & \rowcolor{gray!15} ARI (\%) & 59±29 & 69±8 & 54±31 & 52±38 & 49±33 & 19±32 & 0 & 0 & \textbf{77±5} \\
        %\cline{2-11}
        & $Eps$ & .16±.05 & .16±.08 & .26±.24 & .36±.40 & .22±.14 & .42±.28 & 0 & 0 & \textbf{.12±.04} \\
        & $MinPts$ & 73±88 & 64±41 & 121±101 & 69±127 & 99±103 & 183±129 & 0 & 0 & \textbf{33±19} \\
        & No. Cluster & 16±41 & 3±1 & 3±2 & 15±27 & 8±15 & 2±1 & 0 & 0 & \textbf{4±1} \\
        & First Iteration & 24±10 & 39±11 & 29±23 & 24±18 & 22±14 & 11±19 & 0 & 0 & \textbf{23±9} \\
        & All Iteration & 50±0 & 50±0 & 50±0 & 52±0 & 53±0 & 57±0 & 0 & 0 & \textbf{58±8} \\
        \hline
        \hline
        \multirow{7}*{Aggregation} & \rowcolor{gray!15} NMI (\%) & 65±17 & 59±34 & 45±32 & 52±25 & 64±30 & 45±26 & 0 & 0 & \textbf{96±2} \\
        & \rowcolor{gray!15} AMI (\%) & 64±17 & 59±34 & 45±32 & 40±36 & 63±30 & 44±26 & 0 & 0 & \textbf{96±2} \\
        & \rowcolor{gray!15} ARI (\%) & 51±21 & 54±34 & 39±32 & 33±34 & 56±31 & 35±26 & 0 & 0 & \textbf{96±3} \\
        %\cline{2-11}
        & $Eps$ & .17±.06 & .17±.08 & .34±.25 & 18±20 & .17±.12 & .34±.25 & 0 & 0 & \textbf{.09±.02} \\
        & $MinPts$ & 115±73 & 182±184 & 281±211 & 167±221 & 175±209 & 232±161 & 0 & 0 & \textbf{32±12} \\
        & No. Cluster & 4±2 & 4±2 & 3±1 & 238±379 & 4±2 & 3±1 & 0 & 0 & \textbf{8±1} \\
        & First Iteration & 20±11 & 22±15 & 30±17 & 26±17 & 26±15 & 24±21 & 0 & 0 & \textbf{24±6} \\
        & All Iteration & 50±0 & 50±0 & 50±0 & 52±0 & 53±0 & 57±0 & 0 & 0 & \textbf{44±9} \\
        \hline
        \hline
        \multirow{7}*{D31} & \rowcolor{gray!15} NMI (\%) & 17±16 & 16±15 & 32±28 & 21±19 & 24±23 & 3±6 & 0 & 0 & \textbf{59±21} \\
        & \rowcolor{gray!15} AMI (\%) & 17±16 & 16±15 & 31±28 & 15±15 & 24±23 & 3±6 & 0 & 0 & \textbf{59±21} \\
        & \rowcolor{gray!15} ARI (\%) & 2±4 & 2±3 & 11±18 & 2±3 & 6±10 & 0±0 & 0 & 0 & \textbf{23±9} \\
        %\cline{2-11}
        & $Eps$ & .27±.14 & .41±.18 & .33±.23 & 0.31±.22 & .30±.15 & .47±.34 & 0 & 0 & \textbf{.14±.12} \\
        & $MinPts$ & 1269±911 & 1600±676 & 845±639 & 1599±928 & 1213±851 & 1290±814 & 0 & 0 & \textbf{191±83} \\
        & No. Cluster & 2±1 & 2±1 & 4±6 & 311±979 & 3±4 & 1±1 & 0 & 0 & \textbf{7±3} \\
        & First Iteration & 19±15 & 23±18 & 25±21 & 25±20 & 34±19 & 4±9 & 0 & 0 & \textbf{27±12} \\
        & All Iteration & 50±0 & 50±0 & 50±0 & 52±0 & 53±0 & 57±0 & 0 & 0 & \textbf{46±12} \\
        \hline
        \hline
        \multirow{7}*{IRIS} & \rowcolor{gray!15} NMI (\%) & 0 & 0 & 0 & 0 & 0 & 0 & 0 & 0 & \textbf{0} \\
        & \rowcolor{gray!15} AMI (\%) & 0 & 0 & 0 & 0 & 0 & 0 & 0 & 0 & \textbf{0} \\
        & \rowcolor{gray!15} ARI (\%) & 0 & 0 & 0 & 0 & 0 & 0 & 0 & 0 & \textbf{0} \\
        %\cline{2-11}
        & $Eps$ & 0 & 0 & 0 & 0 & 0 & 0 & 0 & 0 & \textbf{0} \\
        & $MinPts$ & 0 & 0 & 0 & 0 & 0 & 0 & 0 & 0 & \textbf{0} \\
        & No. Cluster & 0 & 0 & 0 & 0 & 0 & 0 & 0 & 0 & \textbf{0} \\
        & First Iteration & 0 & 0 & 0 & 0 & 0 & 0 & 0 & 0 & \textbf{0} \\
        & All Iteration & 50±0 & 50±0 & 50±0 & 52±0 & 53±0 & 57±0 & 0 & 0 & \textbf{0} \\
        \hline
        \hline
        \end{tabular}
    }
\end{table*}

\begin{figure*}[t]
\centering
\subfigure[Pathbased.]{\label{fig:date1-b1}
\begin{minipage}[t]{0.22\linewidth}
\centering
\includegraphics[width=4.2cm]{figures/results/Epoch-NMI(Pathbased).pdf}
\end{minipage}%
}%
\subfigure[Compound.]{\label{fig:date1-b2}
\begin{minipage}[t]{0.22\linewidth}
\centering
\includegraphics[width=4.2cm]{figures/results/Epoch-NMI(Compound).pdf}
\end{minipage}%
}%
\centering
\subfigure[Aggregation.]{\label{fig:date1-b3}
\begin{minipage}[t]{0.22\linewidth}
\centering
\includegraphics[width=4.2cm]{figures/results/Epoch-NMI(Aggregation).pdf}
\end{minipage}%
}%
\centering
\subfigure[D31.]{\label{fig:date2-b1}
\begin{minipage}[t]{0.22\linewidth}
\centering
\includegraphics[width=4.2cm]{figures/results/Epoch-NMI(Aggregation).pdf}
\end{minipage}%
}%
\centering
\caption{Online clustering efficiency comparison.}\label{fig:online}
\end{figure*}

\begin{table*}[t]
    \setlength{\abovecaptionskip}{0.cm}
    \setlength{\belowcaptionskip}{-0.cm}
    \caption{The comparison results of different parameter search method.}\label{tab:complexity}
    \centering
    \scalebox{1.0}{
        \begin{tabular}{c|c|cc|cccc|cc|cc}
        \hline
        \multirow{2}*{\textbf{Dataset}} & \multirow{2}*{\textbf{Metrics}} & \multicolumn{2}{c|}{\textbf{Traditional}} & \multicolumn{4}{c|}{\textbf{Evolutionary}} & \multicolumn{4}{c}{\textbf{Dedicated}} \\
        \cline{3-12}
         &  & \multirow{1}*{\textbf{Rand}} & \multirow{1}*{\textbf{BO-TPE}} & \multirow{1}*{\textbf{Anneal}} & \multirow{1}*{\textbf{PSO}} & \multirow{1}*{\textbf{GA}} & \multirow{1}*{\textbf{DE}} & \multirow{1}*{\textbf{KDist}} & \multirow{1}*{\textbf{BDE}}  & \multirow{1}*{\textbf{DRL_{s}}} & \multirow{1}*{\textbf{DRL_{m}}} \\
        \hline
        \hline 
        \multirow{7}*{ALL} & \rowcolor{gray!15} NMI (\%) & 61±24 & 80±5 & 57±39 & 52±41 & 12±9 & 6±8 & 0 & 0 & 0 & \textbf{0} \\
        & \rowcolor{gray!15} AMI (\%) & 17±24 & 30±37 & 49±34 & 30±35 & 11±8 & 5±7 & 0 & 0 & 0 & \textbf{0} \\
        & \rowcolor{gray!15} ARI (\%) & 2±5 & 19±27 & 20±22 & 22±29 & 1±1 & 1±1 & 0 & 0 & 0 & \textbf{0} \\
        %\cline{2-12}
        & $Eps$ & .72±.36 & .63±.37 & 3.4±4.3 & 3.4±4.6 & 3.3±3.5 & 5.9±4.3 & 0 & 0 & 0 & \textbf{0} \\
        & $MinPts$ & 2±1 & 1±1 & 2±1 & 106±149 & 260±152 & 274±113 & 0 & 0 & 0 & \textbf{0} \\
        & No. of Cluster & 835±801 & 1117±618 & 165±203 & 552±615 & 2±1 & 2±1 & 0 & 0 & 0 & \textbf{0} \\
        & First Iteration & 25±14 & 26±11 & 24±19 & 24±21 & 20±17 & 13±18 & 0 & 0 & \textbf{0} & \textbf{0} \\
        & All Iteration & 50±0 & 50±0 & 50±0 & 52±0 & 53±0 & 57±0 & 0 & 0 & \textbf{0} & \textbf{0}\\
        \hline
        \hline
        \multirow{7}*{Shape} & \rowcolor{gray!15} NMI (\%) & 35±29 & 57±21 & 14±19 & 53±29 & 19±2 & 7±6 & 0 & 0 & 0 & \textbf{0} \\
        & \rowcolor{gray!15} AMI (\%) & 14±13 & 15±13 & 9±12 & 7±9 & 18±2 & 6±5 & 0 & 0 & 0 & \textbf{0} \\
        & \rowcolor{gray!15} ARI (\%) & 2±3 & 2±2 & 1±1 & 1±1 & 1±0 & 0±0 & 0 & 0 & 0 & \textbf{0} \\
        %\cline{2-12}
        & $Eps$ & .24±.21 & .09±.05 & 3.3±3.1 & .19±.25 & .46.10 & 1.7±2.2 & 0 & 0 & 0 & \textbf{0} \\
        & $MinPts$ & 2±1 & 2±1 & 3±1 & 159±204 & 295±134 & 201±117 & 0 & 0 & 0 & \textbf{0} \\
        & No. of Cluster & 378±577 & 790±795 & 26±38 & 960±825 & 2±0 & 2±0 & 0 & 0 & 0 & \textbf{0} \\
        & First Iteration & 23±14 & 28±9 & 13±19 & 20±13 & 26±15 & 22±18 & 0 & 0 & \textbf{0} & \textbf{0} \\
        & All Iteration & 50±0 & 50±0 & 50±0 & 52±0 & 53±0 & 57±0 & 0 & 0 & \textbf{0} & \textbf{0} \\
        \hline
        \hline
        \multirow{7}*{Texture} & \rowcolor{gray!15} NMI (\%) & 64±24 & 73±8 & 30±34 & 34±37 & 12±14 & 3±5 & 0 & 0 & 0 & \textbf{0} \\
        & \rowcolor{gray!15} AMI (\%) & 14±14 & 17±17 & 15±17 & 4±5 & 9±7 & 2±5 & 0 & 0 & 0 & \textbf{0} \\
        & \rowcolor{gray!15} ARI (\%) & 4±5 & 6±9 & 5±9 & 1±1 & 1±0 & 0±0 & 0 & 0 & 0 & \textbf{0} \\
        %\cline{2-12}
        & $Eps$ & .34±.22 & .28±.14 & 3.5±3.3 & 2.0±2.6 & .93±.51 & 3.7±2.8 & 0 & 0 & 0 & \textbf{0} \\
        & $MinPts$ & 2±1 & 1±0 & 2±1 & 112±143 & 297±126 & 159±118 & 0 & 0 & 0 & \textbf{0} \\
        & No. of Cluster & 1042±689 & 1165±574 & 252±454 & 628±810 & 31±95 & 1±1 & 0 & 0 & 0 & \textbf{0} \\
        & First Iteration & 21±17 & 27±12 & 19±21 & 20±18 & 30±18 & 4±6 & 0 & 0 & \textbf{0} & \textbf{0} \\
        & All Iteration & 50±0 & 50±0 & 50±0 & 52±0 & 53±0 & 57±0 & 0 & 0 & \textbf{0} & \textbf{0} \\
        \hline
        \hline
        \multirow{7}*{Margin} & \rowcolor{gray!15} NMI (\%) & 51±25 & 70±14 & 42±31 & 16±22 & 17±6 & 10±14 & 0 & 0 & 0 & 0  \\
        & \rowcolor{gray!15} AMI (\%) & 22±16 & 6±13 & 14±18 & 8±8 & 16±6 & 9±12 & 0 & 0 & 0 & 0 \\
        & \rowcolor{gray!15} ARI (\%) & 2±3 & 0±1 & 1±1 & 1±1 & 1±1 & 1±1 & 0 & 0 & 0 & 0 \\
        %\cline{2-12}
        & $Eps$ & .60±.16 & .27±.21 & 1.9±2.4 & 2.0±1.7 & 1.1±.16 & 2.7±1.9 & 0 & 0 & 0 & 0 \\
        & $MinPts$ & 2±1 & 1±1 & 2±1 & 173±124 & 258±152 & 121±61 & 0 & 0 & 0 & 0 \\
        & No. of Cluster & 537±672 & 1291±648 & 503±744 & 161±505 & 2±1 & 3±5 & 0 & 0 & 0 & 0 \\
        & First Iteration & 23±12 & 23±12 & 19±17 & 23±23 & 19±11 & 9±19 & 0 & 0 & \textbf{0} & 0 \\
        & All Iteration & 50±0 & 50±0 & 50±0 & 52±0 & 53±0 & 57±0 & 0 & 0 & \textbf{0} & 0 \\
        \hline
        \hline
        \end{tabular}
    }
\end{table*}

\begin{table}[t]
    \setlength{\abovecaptionskip}{0.cm}
    \setlength{\belowcaptionskip}{-0.cm}
    \caption{Multi-dimensional results.}\label{tab:multi-dimensional}
    \centering
    \scalebox{1.0}{
        \begin{tabular}{c|cc|cc}
        \hline
        \multirow{2}*{\textbf{Method}} & \multicolumn{2}{c|}{\textbf{Reuters}} & \multicolumn{2}{c}{\textbf{100 leaves}}\\
        \cline{2-5}
         & NMI (\%) & Iteration & NMI (\%) & Iteration\\
        \hline
        GA & 0 & 0 & 0 & 0  \\
        PSO & 0 & 0 & 0 & 0  \\
        ACO & 0 & 0 & 0 & 0  \\
        \hline
        SMAC & 0 & 0 & 0 & 0  \\
        Randomly & 0 & 0 & 0 & 0  \\
        \hline
        V-DBSCAN & 0 & 0 & 0 & 0  \\
        BDE-DBSCAN & 0 & 0 & 0 & 0  \\
        \hline
        {\framework}* & 0 & 0 & 0 & 0\\
        {\framework} & 0 & 0 & 0 & 0 \\
        \hline
        \end{tabular}
    }
\end{table}

\begin{figure*}[t]
\centering
\subfigure[Data 1 Block 1.]{\label{fig:date1-b1}
\begin{minipage}[t]{0.333\linewidth}
\centering
\includegraphics[width=5.3cm]{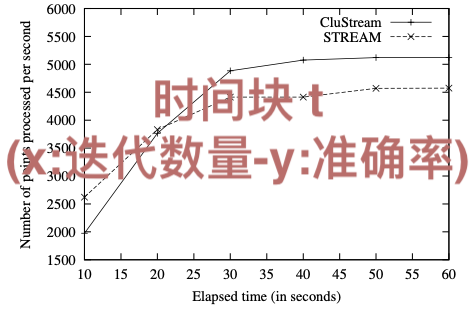}
\end{minipage}%
}%
\subfigure[Data 1 Block 3.]{\label{fig:date1-b2}
\begin{minipage}[t]{0.333\linewidth}
\centering
\includegraphics[width=5.3cm]{}
\end{minipage}%
}%
\centering
\subfigure[Data 1 Block 5.]{\label{fig:date1-b3}
\begin{minipage}[t]{0.333\linewidth}
\centering
\includegraphics[width=5.3cm]{}
\end{minipage}%
}%
\centering

\subfigure[Data 2 Block 1.]{\label{fig:date2-b1}
\begin{minipage}[t]{0.333\linewidth}
\centering
\includegraphics[width=5.3cm]{}
\end{minipage}%
}%
\subfigure[Data 2 Block 3.]{\label{fig:date2-b2}
\begin{minipage}[t]{0.333\linewidth}
\centering
\includegraphics[width=5.3cm]{}
\end{minipage}%
}%
\centering
\subfigure[Data 2 Block 5.]{\label{fig:date2-b3}
\begin{minipage}[t]{0.333\linewidth}
\centering
\includegraphics[width=5.3cm]{}
\end{minipage}%
}%
\centering
\caption{Online clustering efficiency comparison.}\label{fig:online}
\end{figure*}

\begin{table*}[t]
    \setlength{\abovecaptionskip}{0.cm}
    \setlength{\belowcaptionskip}{-0.cm}
    \caption{Online evaluation and comparison in Predictive Mode.}\label{tab:complexity}
    \centering
    \scalebox{1.0}{
        \begin{tabular}{c|c|cc|cccc|cc|cc}
        \hline
        \multirow{2}*{\textbf{Chunks}} & \multirow{2}*{\textbf{Metrics}} & \multicolumn{2}{c|}{\textbf{Traditional}} & \multicolumn{4}{c|}{\textbf{Evolutionary}} & \multicolumn{4}{c}{\textbf{Dedicated}} \\
        \cline{3-12}
         & & \multirow{1}*{\textbf{Rand}} & \multirow{1}*{\textbf{BO-TPE}} & \multirow{1}*{\textbf{Anneal}} & \multirow{1}*{\textbf{PSO}} & \multirow{1}*{\textbf{GA}} & \multirow{1}*{\textbf{DE}} & \multirow{1}*{\textbf{KDist}} & \multirow{1}*{\textbf{BDE}} & \multirow{1}*{\textbf{DRL_{p}}} & \multirow{1}*{\textbf{DRL_{t}}}\\
        \hline
        \hline 
        \rowcolor{gray!15} $\mathcal{V}_{1}$ & NMI & .73±.19 & .86±.03 & .00±.00 & .00±.00 & .00±.00 & .00±.00 & .00±.00 & .00±.00 & \textbf{.09±.27} & \textbf{.91±.02} \\
        \rowcolor{white!15}                  & ARI & .39±.33 & .59±.15 & .00±.00 & .00±.00 & .00±.00 & .00±.00 & .00±.00 & .00±.00 & \textbf{.06±.19} & \textbf{.76±.03} \\
        \rowcolor{gray!15} $\mathcal{V}_{2}$ & NMI & .88±.04 & .91±.02 & .00±.00 & .00±.00 & .00±.00 & .00±.00 & .00±.00 & .00±.00 & \textbf{.85±.12} & \textbf{.94±.00} \\
        \rowcolor{white!15}                  & ARI & .61±.18 & .74±.12 & .00±.00 & .00±.00 & .00±.00 & .00±.00 & .00±.00 & .00±.00 & \textbf{.55±.26} & \textbf{.85±.00} \\
        \rowcolor{gray!15} $\mathcal{V}_{3}$ & NMI & .90±.06 & .94±.01 & .00±.00 & .00±.00 & .00±.00 & .00±.00 & .00±.00 & .00±.00 & \textbf{.87±.07} & \textbf{.96±.00} \\
        \rowcolor{white!15}                  & ARI & .68±.25 & .83±.03 & .00±.00 & .00±.00 & .00±.00 & .00±.00 & .00±.00 & .00±.00 & \textbf{.58±.23} & \textbf{.85±.00} \\
        \rowcolor{gray!15} $\mathcal{V}_{4}$ & NMI & .88±.08 & .92±.02 & .00±.00 & .00±.00 & .00±.00 & .00±.00 & .00±.00 & .00±.00 & \textbf{.90±.04} & \textbf{.93±.00} \\
        \rowcolor{white!15}                  & ARI & .64±.22 & .72±.07 & .00±.00 & .00±.00 & .00±.00 & .00±.00 & .00±.00 & .00±.00 & \textbf{.69±.16} & \textbf{.76±.02} \\
        \rowcolor{gray!15} $\mathcal{V}_{5}$ & NMI & .36±.16 & .53±.16 & .00±.00 & .00±.00 & .00±.00 & .00±.00 & .00±.00 & .00±.00 & \textbf{.13±.05} & \textbf{.00±.00} \\
        \rowcolor{white!15}                  & ARI & .02±.02 & .08±.06 & .00±.00 & .00±.00 & .00±.00 & .00±.00 & .00±.00 & .00±.00 & \textbf{.00±.00} & \textbf{.00±.00} \\
        \rowcolor{gray!15} $\mathcal{V}_{6}$ & NMI & .83±.08 & .89±.01 & .00±.00 & .00±.00 & .00±.00 & .00±.00 & .00±.00 & .00±.00 & \textbf{.83±.05} & \textbf{.91±.00} \\
        \rowcolor{white!15}                  & ARI & .50±.20 & .66±.07 & .00±.00 & .00±.00 & .00±.00 & .00±.00 & .00±.00 & .00±.00 & \textbf{.43±.16} & \textbf{.71±.00} \\
        \rowcolor{gray!15} $\mathcal{V}_{7}$ & NMI & .84±.05 & .86±.01 & .00±.00 & .00±.00 & .00±.00 & .00±.00 & .00±.00 & .00±.00 & \textbf{.84±.02} & \textbf{.01±.00} \\
        \rowcolor{white!15}                  & ARI & .48±.11 & .51±.02 & .00±.00 & .00±.00 & .00±.00 & .00±.00 & .00±.00 & .00±.00 & \textbf{.45±.07} & \textbf{.00±.00} \\
        \rowcolor{gray!15} $\mathcal{V}_{8}$ & NMI & .85±.04 & .87±.01 & .00±.00 & .00±.00 & .00±.00 & .00±.00 & .00±.00 & .00±.00 & \textbf{.00±.00} & \textbf{.88±.00} \\
        \rowcolor{white!15}                  & ARI & .46±.10 & .50±.07 & .00±.00 & .00±.00 & .00±.00 & .00±.00 & .00±.00 & .00±.00 & \textbf{.00±.00} & \textbf{.48±.04} \\
        \hline
        \hline
        \end{tabular}
    }
\end{table*}

\subsection{Multi-dimension DBSCAN Clustering Algorithm}\label{sec:multi-dimension}
In practical applications, the globally fixed density parameter is often only suitable for \tobeupdated{low-dimensional \cite{}} or some \tobeupdated{uniform density \cite{} data}.
In high-dimensional data, the curse of dimensionality of DBSCAN can lead to sparsity in the sample space.
In addition, when there are significant density differences between dimensions, different (group) dimensions require individualized density parameters.
To this end, we propose an improved DBSCAN algorithm with personalized parameters.
Specifically, we improve the definition of Direct Density-reachable in DBSCAN as follows:

\begin{define}
    \textbf{(Directly Density-reachable in Multi-dimensional Clustering).} 
    An object $v_{j}$ is directly density reachable from another object $v_{i}$ in multi-dimension data chunk $\mathcal{V}$ if $\forall \mathcal{X}_p \in \{\mathcal{X}_{1},...,\mathcal{X}_{p},\mathcal{X}_{p+1},...\}$:
    \begin{enumerate}
        \item [1)] $v_{j} \in N_{Eps_p}(v_{i})$,
        \item [2)] $v_{i}$ is the core point.
    \end{enumerate}
    Here, $N_{Eps_p}(v_{i})$ represents the set of points in chunk $\mathcal{V}$ that are less than distance $Eps_p$ from $v_{i}$.
    Note that the distance here is the Euclidean distance calculated with the feature group $\mathcal{X}_p$.
    And the condition for an object to be the core point in the feature group $\mathcal{X}_p$ is $|N_{Eps_p}(v_{i})| \geq {Minpts}_{p}$.
\end{define}

The other clustering steps (Density-reachable, Density-connected, and Cluster) of our improved DBSCAN algorithm suitable for multi-dimensional clustering are the same as those of the original DBSCAN algorithm, which will not be repeated here.

\begin{figure}[t]
\centering
\includegraphics[width=8.5cm]{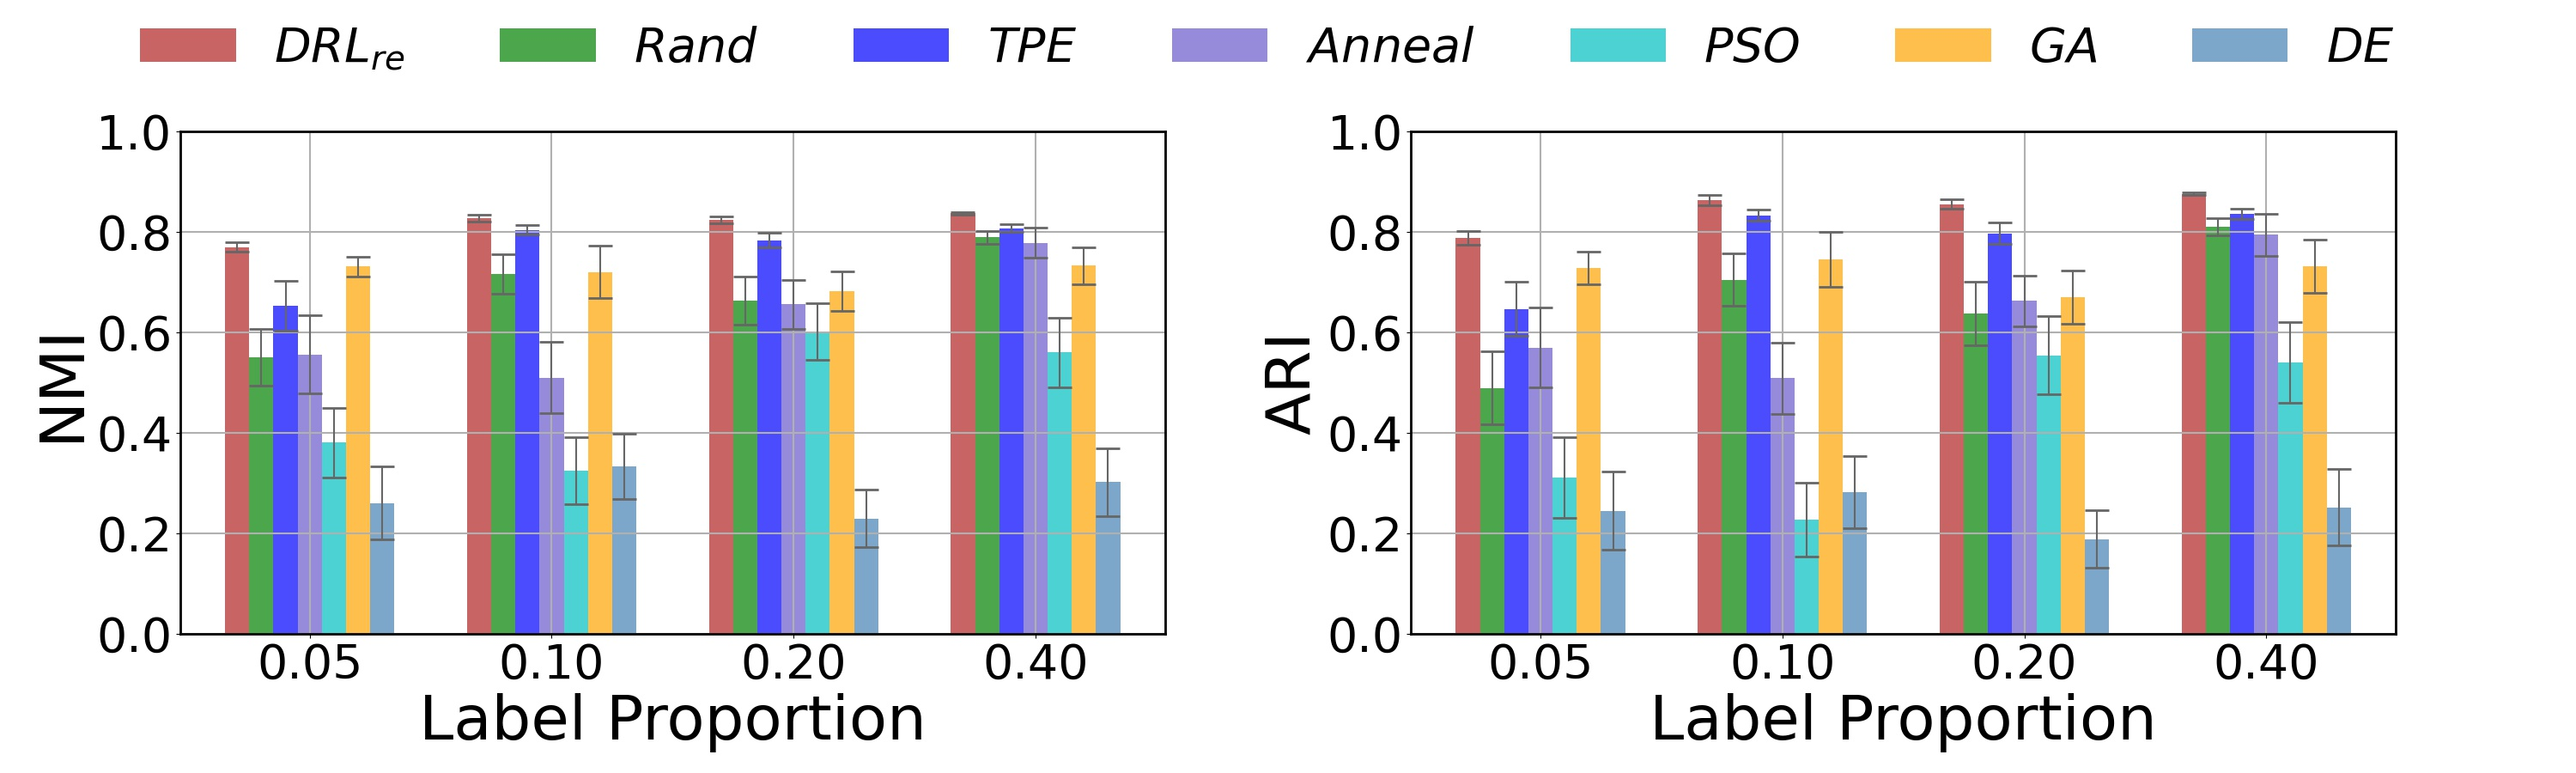}\vspace{-1em}
\centering
\caption{Label percentage.}\label{fig:percentage}
\end{figure}

\begin{figure}[t]
\centering
\includegraphics[width=8.5cm]{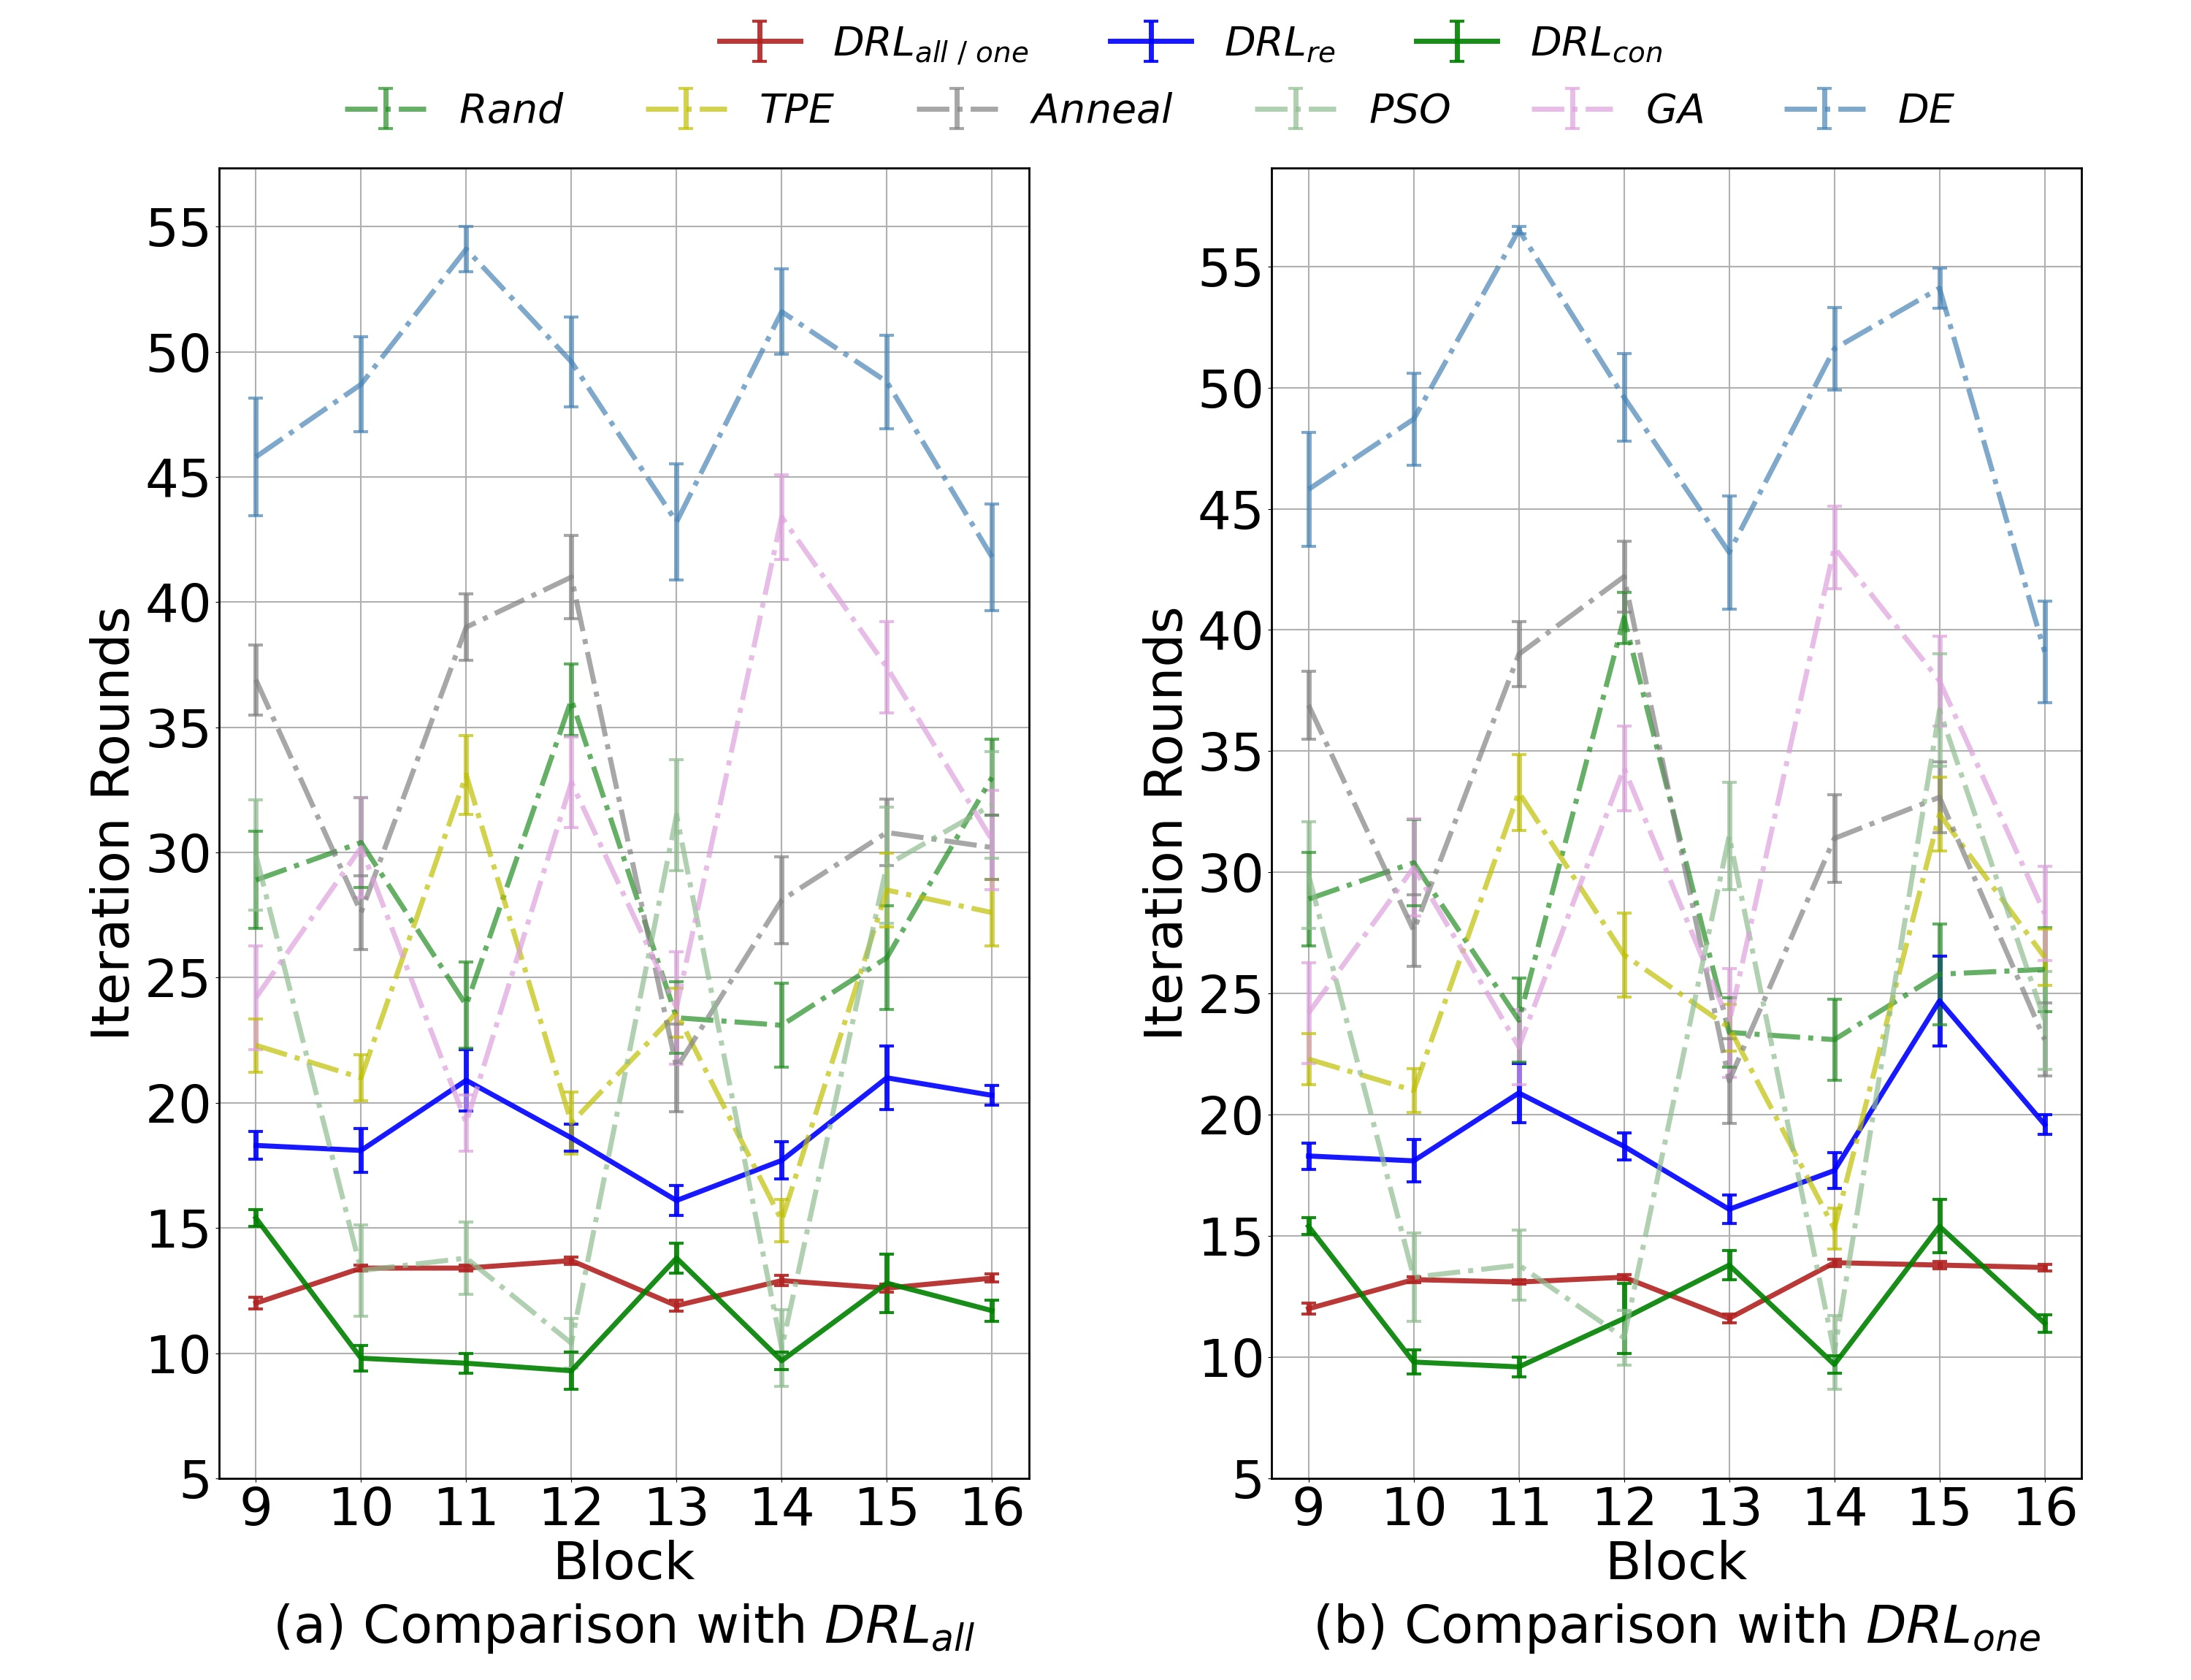}\vspace{-1em}
\centering
\caption{Comparison of online task round consumption.}\label{fig:online}
\end{figure}

\begin{figure}[t]
\centering
\includegraphics[width=8.5cm]{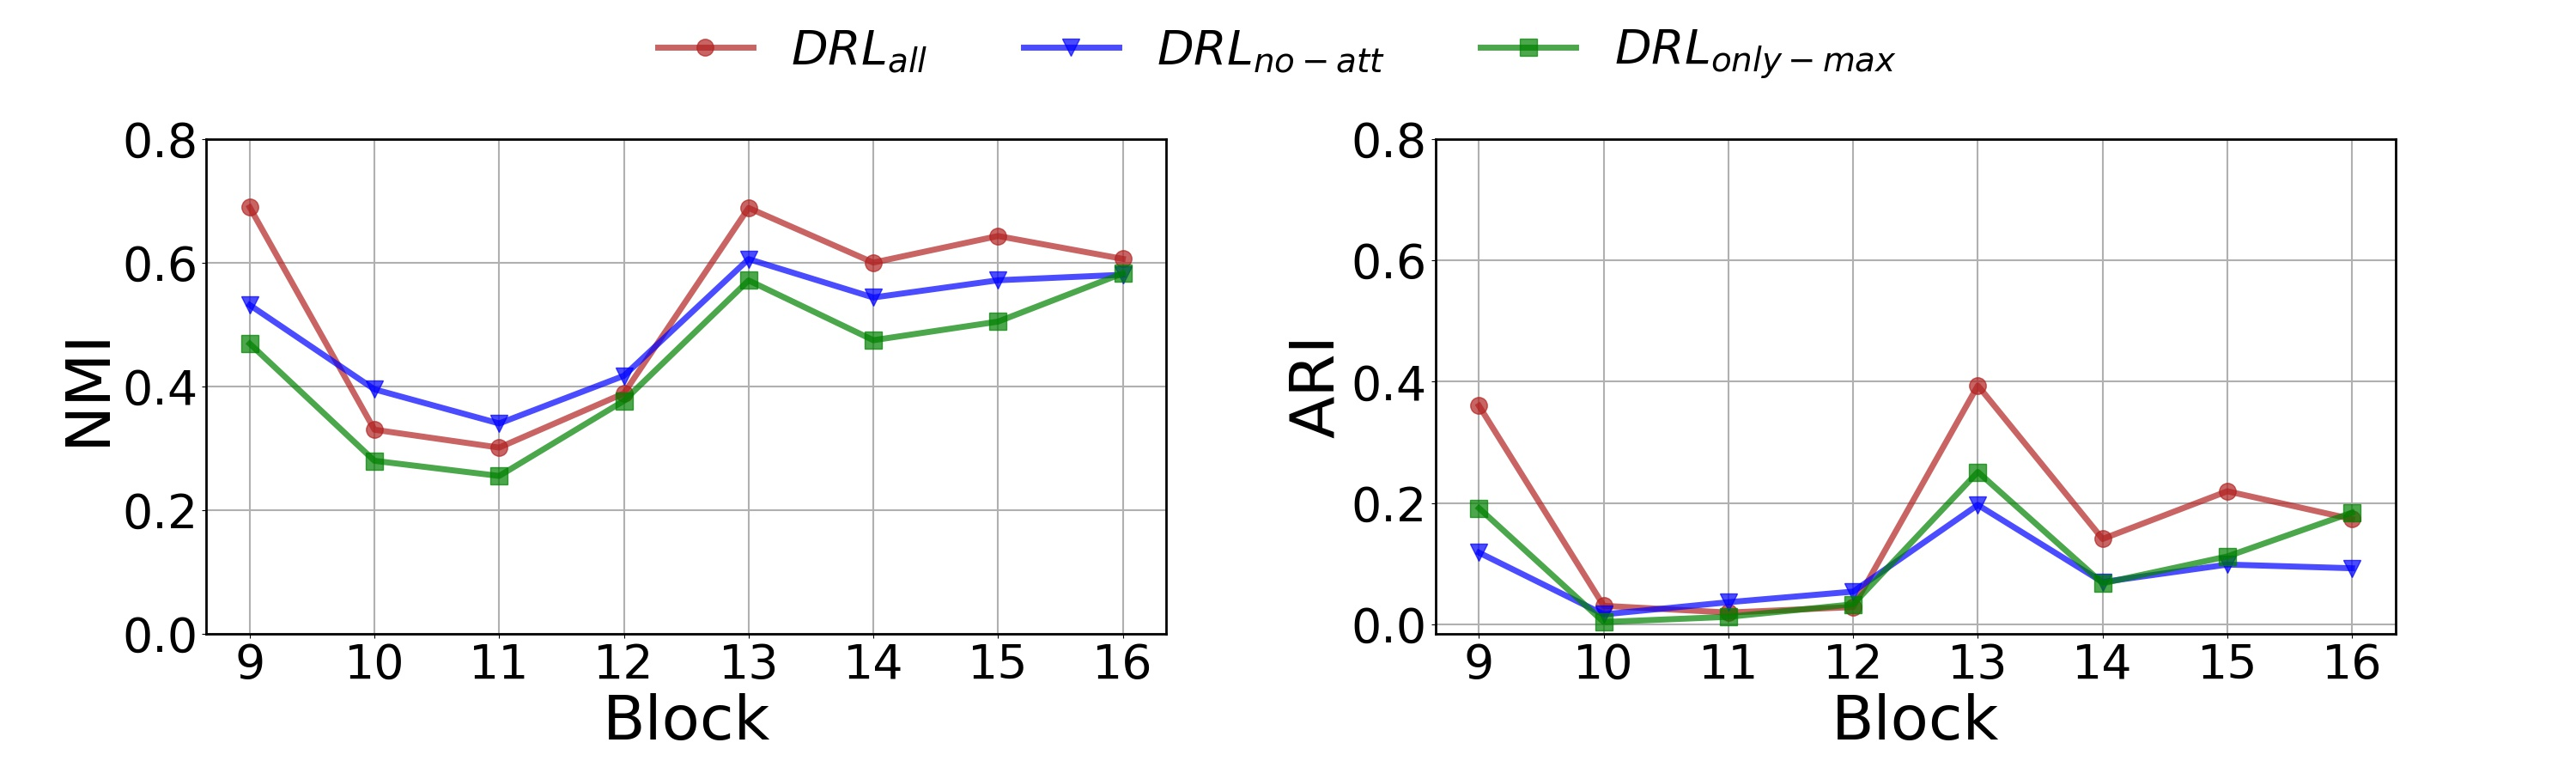}\vspace{-1em}
\centering
\caption{Performance of model variants in online evaluation.}\label{fig:variants}
\end{figure}
